# Supplementary material for: Analysing Russian Trolls via NLP tools
Source: arXiv:1911.11067 source file (2019-11-11)
Supplement: Supplementary file 1 [file appendix3.tex]

\chapter*{Appendix 3: Description of Artefact}
\addcontentsline{toc}{chapter}{Appendix 3: Description of Artefact}
\vspace{-1em}

The code repository contains three folders and other csv files and jupyter notebook files, which is shown in figure~\ref{fig:c}.\\ 
\begin{figure}[h]
	\centering
	\includegraphics[width=\textwidth]{{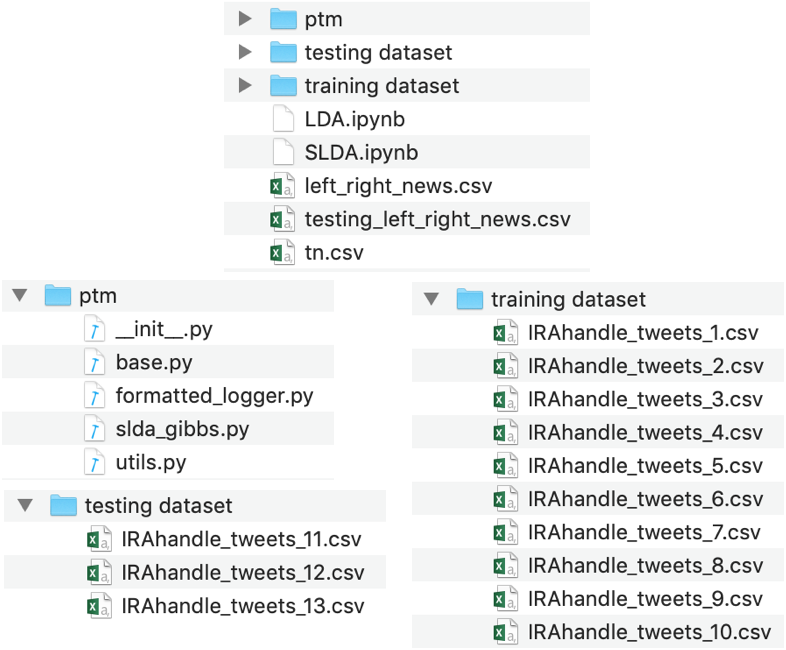}}
	\caption{List of code.}
	\label{fig:c}
\end{figure}\\
\begin{enumerate}
    \item \textbf{"ptm"} includes .py files for the algorithms of supervised topic model implemented in this research. Code files in "ptm" are taken from my supervisor Dr. Dongwoo Kim\footnote{Link to code files: https://github.com/dongwookim-ml/python-topic-model/tree/master/ptm}.
    \item Folder \textbf{"training dataset"}, and \textbf{"testing dataset"} are Russian trolls dataset used in this reseach, the original dataset\footnote{Link to the dataset: https://github.com/fivethirtyeight/russian-troll-tweets/} has 13 separated csv files, and we manually separate the first 10 csv files to training dataset, and the last 3 csv files to testing dataset.
    
    \item \textbf{"tn.csv"} is the publicly available Twitter dataset that we used to train the sentiment model in this research, and the dataset is provided on kaggle\footnote{Link to kaggle dataset: https://www.kaggle.com/kazanova/sentiment140}.
    
    \item \textbf{"left\_right\_news.csv"} and \textbf{"testing\_left\_right\_news.csv"} are pre-processed dataset generated from original Russian troll dataset. The implementation of pre-processing procedure is implemented by myself in jupyter notebook code files.
    
    \item \textbf{"LDA.ipynb"} is the implementation of data pre-processing and topic model, which is implemented by myself.
    
    \item \textbf{"SLDA.ipynb"} is the implementation of data pre-processing, supervised topic model, and sentiment analysis. I make use of sLDA algorithms implemented by Dr. Dongwoo Kim\footnote{Link to code files: https://github.com/dongwookim-ml/python-topic-model/tree/master/ptm}, and I modify the algorithm of sentiment analysis based on an online tutorial\footnote{https://towardsdatascience.com/basic-binary-sentiment-analysis-using-nltk-c94ba17ae386}.
\end{enumerate} 
In terms of experiment setup, we use a laptop computer with configuration as: Intel(R) Core(TM) i7-8750 CPU @ 3.40GHz 3.41GHz; 16.00GB Installed RAM. The codes are developed on jupyter notebook using Anaconda Navigator 1.9.6 with Python 3.7.
