# Supplementary material for: Analysing Russian Trolls via NLP tools
Source: arXiv:1911.11067 source file (2019-11-11)
Supplement: Supplementary file 2 [file appendix4.tex]

\chapter*{Appendix 4: README}
\addcontentsline{toc}{chapter}{Appendix 4: README}
\vspace{-1em}

We analyse the strategies that Russian trolls used in 2016 U.S. Presidential Election from a Twitter dataset containing Russian troll tweets. Various natural language processing techniques are implemented, including topic model, supervised topic model, and sentiment analysis.\\\\\\
{\LARGE Usage}\\\\
{\Large Prerequisites}\\\\
Note: The program can be run on a machine either with or without GPU.
\begin{enumerate}
    \item Install Python 3.7 and Anaconda Navigator containing jupyter notebook.
    \item Install Python libraries: NLTK and gensim which are useful NLP tools.
\end{enumerate}
The Russian troll dataset\footnote{Also can be downloaded from: https://github.com/fivethirtyeight/russian-troll-tweets/} and sentiment analysis dataset\footnote{Also can be downloaded from: https://www.kaggle.com/kazanova/sentiment140} are provided in the uploaded artefact/software.\\\\\\
{\Large Program description}\\
\begin{enumerate}
    \item Firstly open "LDA.ipynb" using jupyter notebook. The "LDA.ipynb" file contains implementations of reading the dataset, extracting usful information and saving a new file, pre-processing the dataset, training the LDA model for topic model using Bag-of-word and tf-idf separately on the Russian troll dataset, representing the result. It can be run individually within a single cell. "LDA.ipynb" will use folder "training dataset", "left\_right\_news.csv".
    \item Secondly open "SLDA.ipynb" using jupyter notebook. The "SLDA.ipynb" file contains implementations of reading the dataset, extracting usful information and saving a new file, pre-processing the dataset, training the sLDA model for supervised topic model using Bag-of-word on the Russian troll dataset, training sLDA model with restricted time range seperately in 2015, 2016, and 2017, training five different sentiment classifiers, predicting sentiments on the Russian troll dataset,  representing the result. It can be run individually within a single cell. "SLDA.ipynb" will use folder "testing dataset", "testing\_left\_right\_news.csv", all python files in folder "ptm", "tn.csv".
\end{enumerate}
