# Supplementary material for: Analysing Russian Trolls via NLP tools
Source: arXiv:1911.11067 source file (2019-11-11)
Supplement: Supplementary file 3 [file appendix1.tex]

\chapter*{Appendix 1: Project Description}
\addcontentsline{toc}{chapter}{Appendix 1: Project Description}
\vspace{-1em}

Natural language processing is a set of method designed to analyse the written natural language corpus. In this project, we will learn about roles of some core NLP tools and how to apply these tools to analyse dataset. Specifically, we will use the existing Twitter dataset published by previous researchers and some of the well-known NLP tools written in Python. The applied NLP tools can be used to summarise the text corpus used in the experiments. For example, topic model can be implemented in this research.\\\\
The specific objective are:
\begin{enumerate}
    \item Learning about how to use python natural language processing (NLP) toolkit.
    \item Learning about how to apply NLP tool to text dataset.
    \item Learning about how to evaluate the result of some NLP methods.
\end{enumerate}
