# Supplementary material for: Analysing Russian Trolls via NLP tools
Source: arXiv:1911.11067 source file (2019-11-11)
Supplement: Supplementary file 4 [file appendix2.tex]

\chapter*{Appendix 2: Study Contract}
\addcontentsline{toc}{chapter}{Appendix 2: Study contract}
\vspace{-1em}

\begin{figure}[h]
	\centering
	\includegraphics[width=\textwidth]{{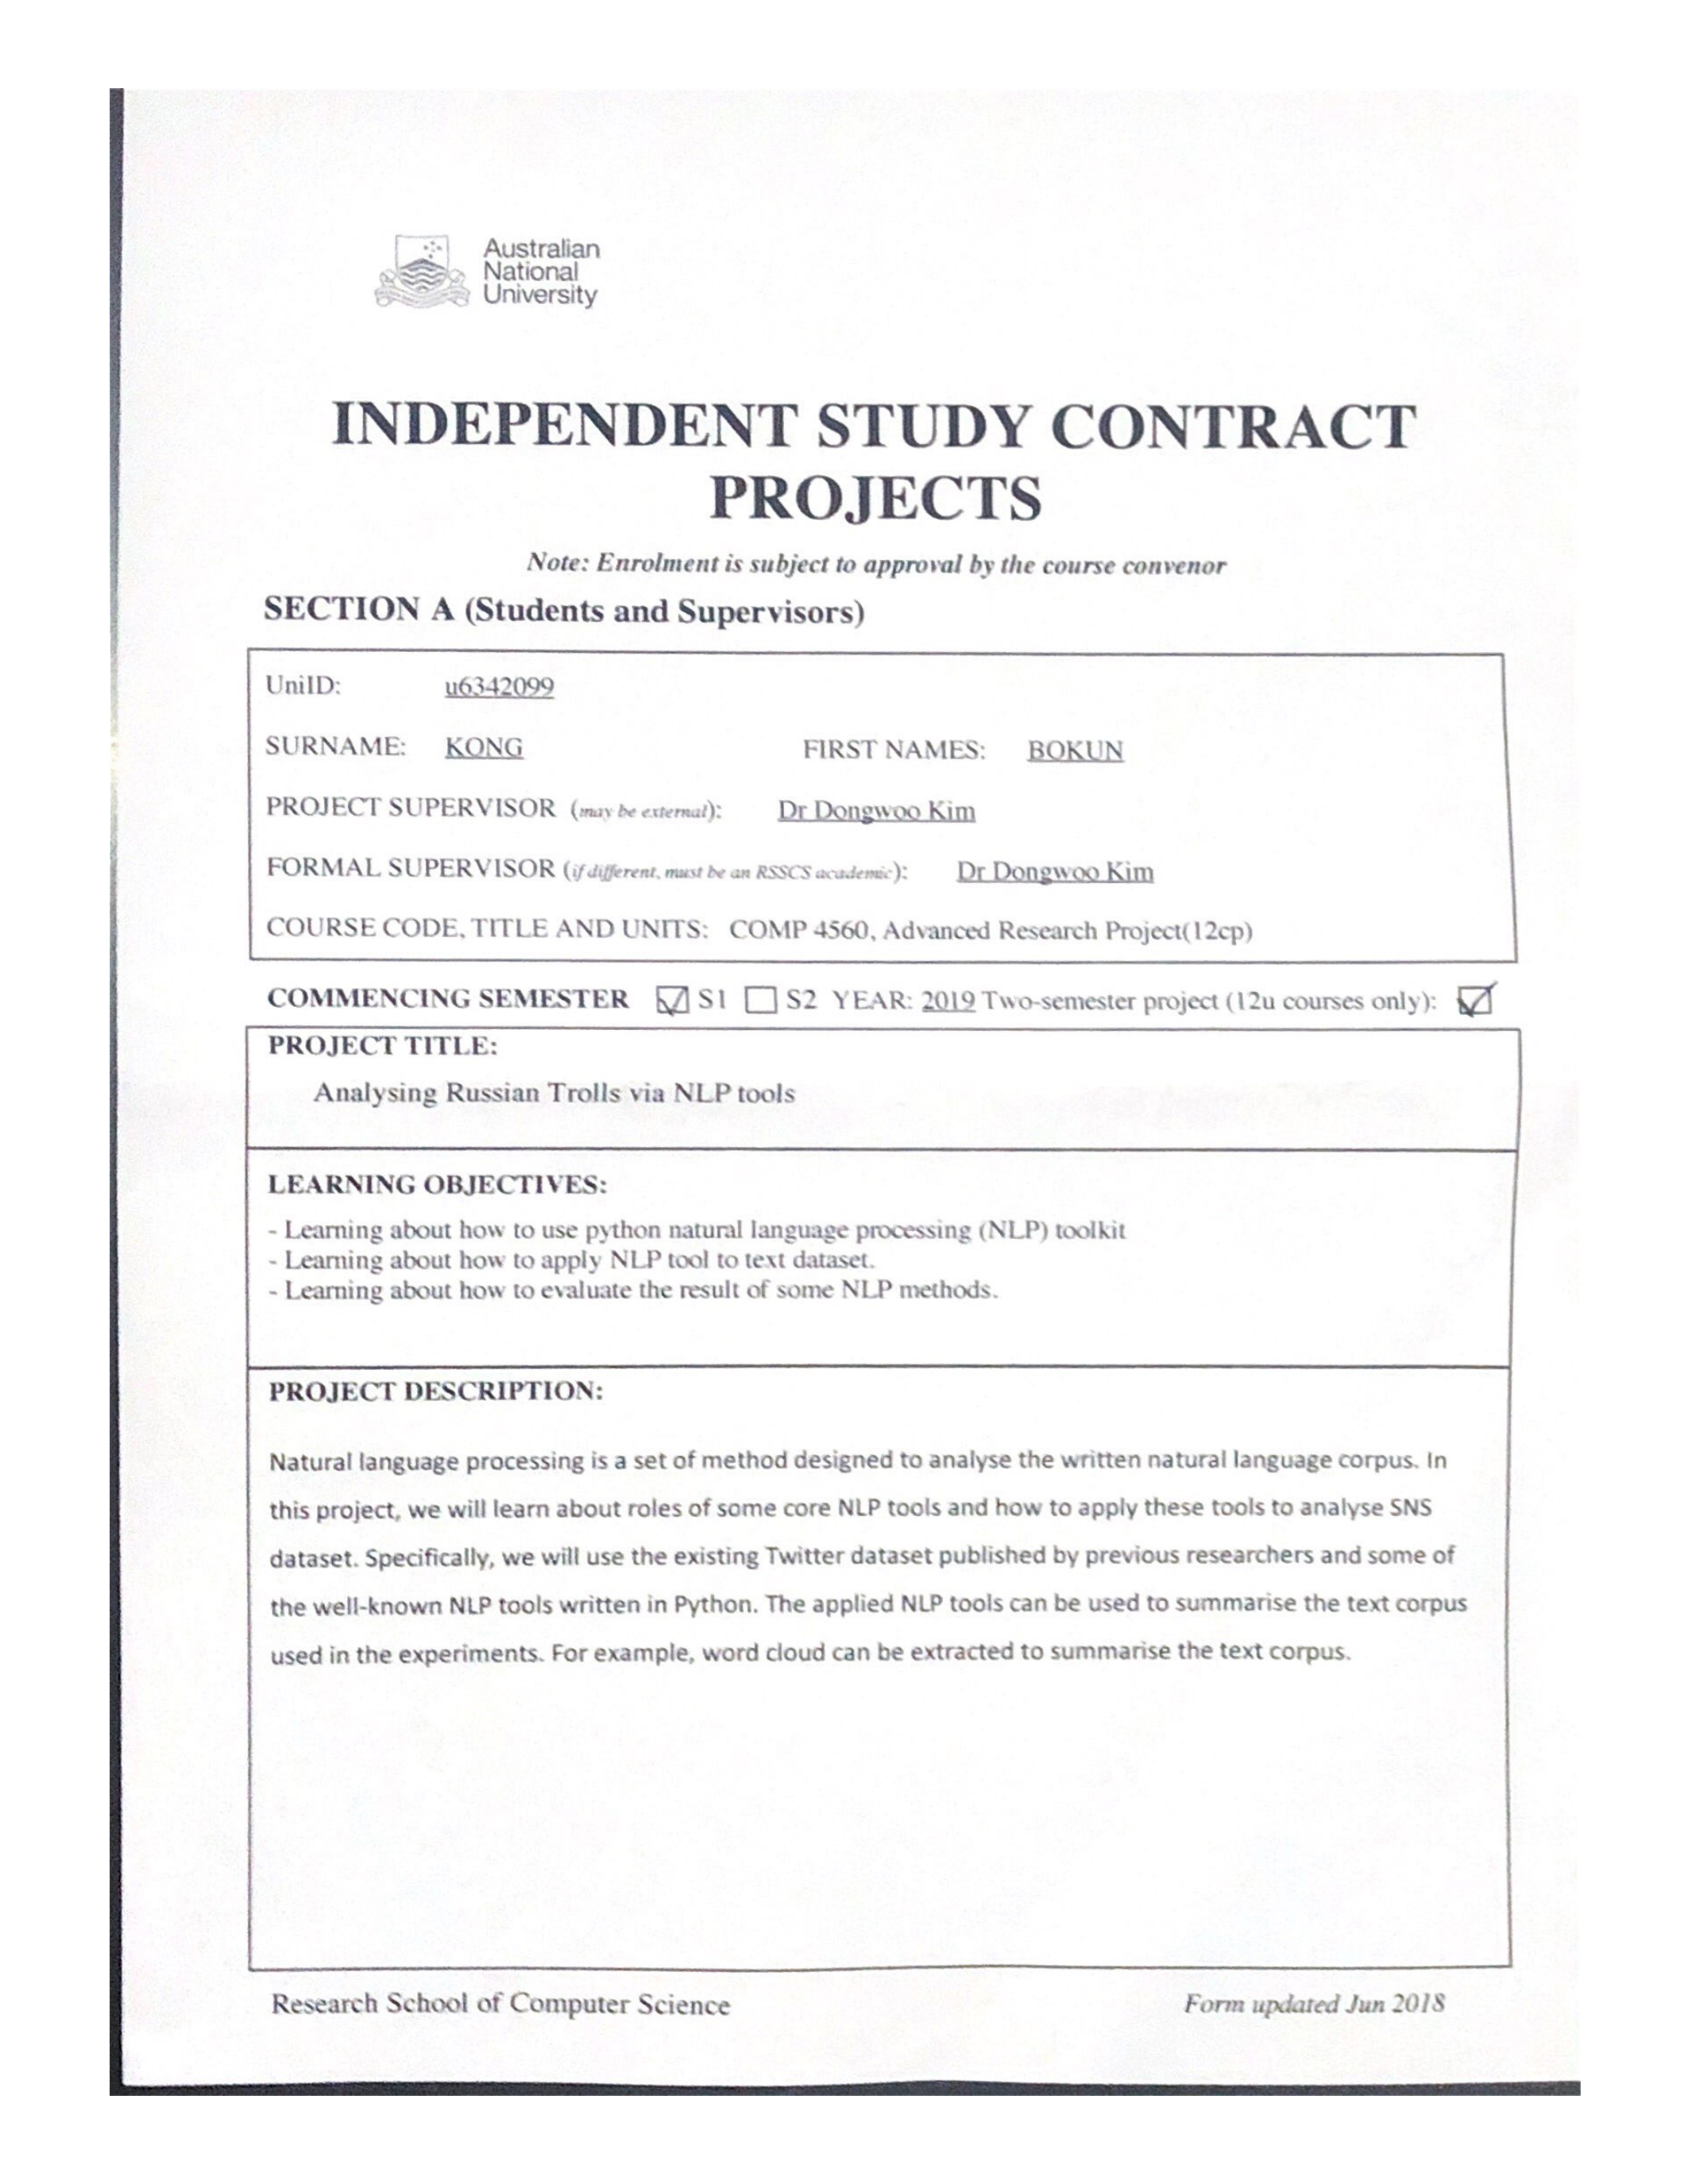}}
	\caption{Independent study contract.}
	\label{fig:ct}
\end{figure}

\begin{figure}[h]
	\centering
	\includegraphics[width=\textwidth]{{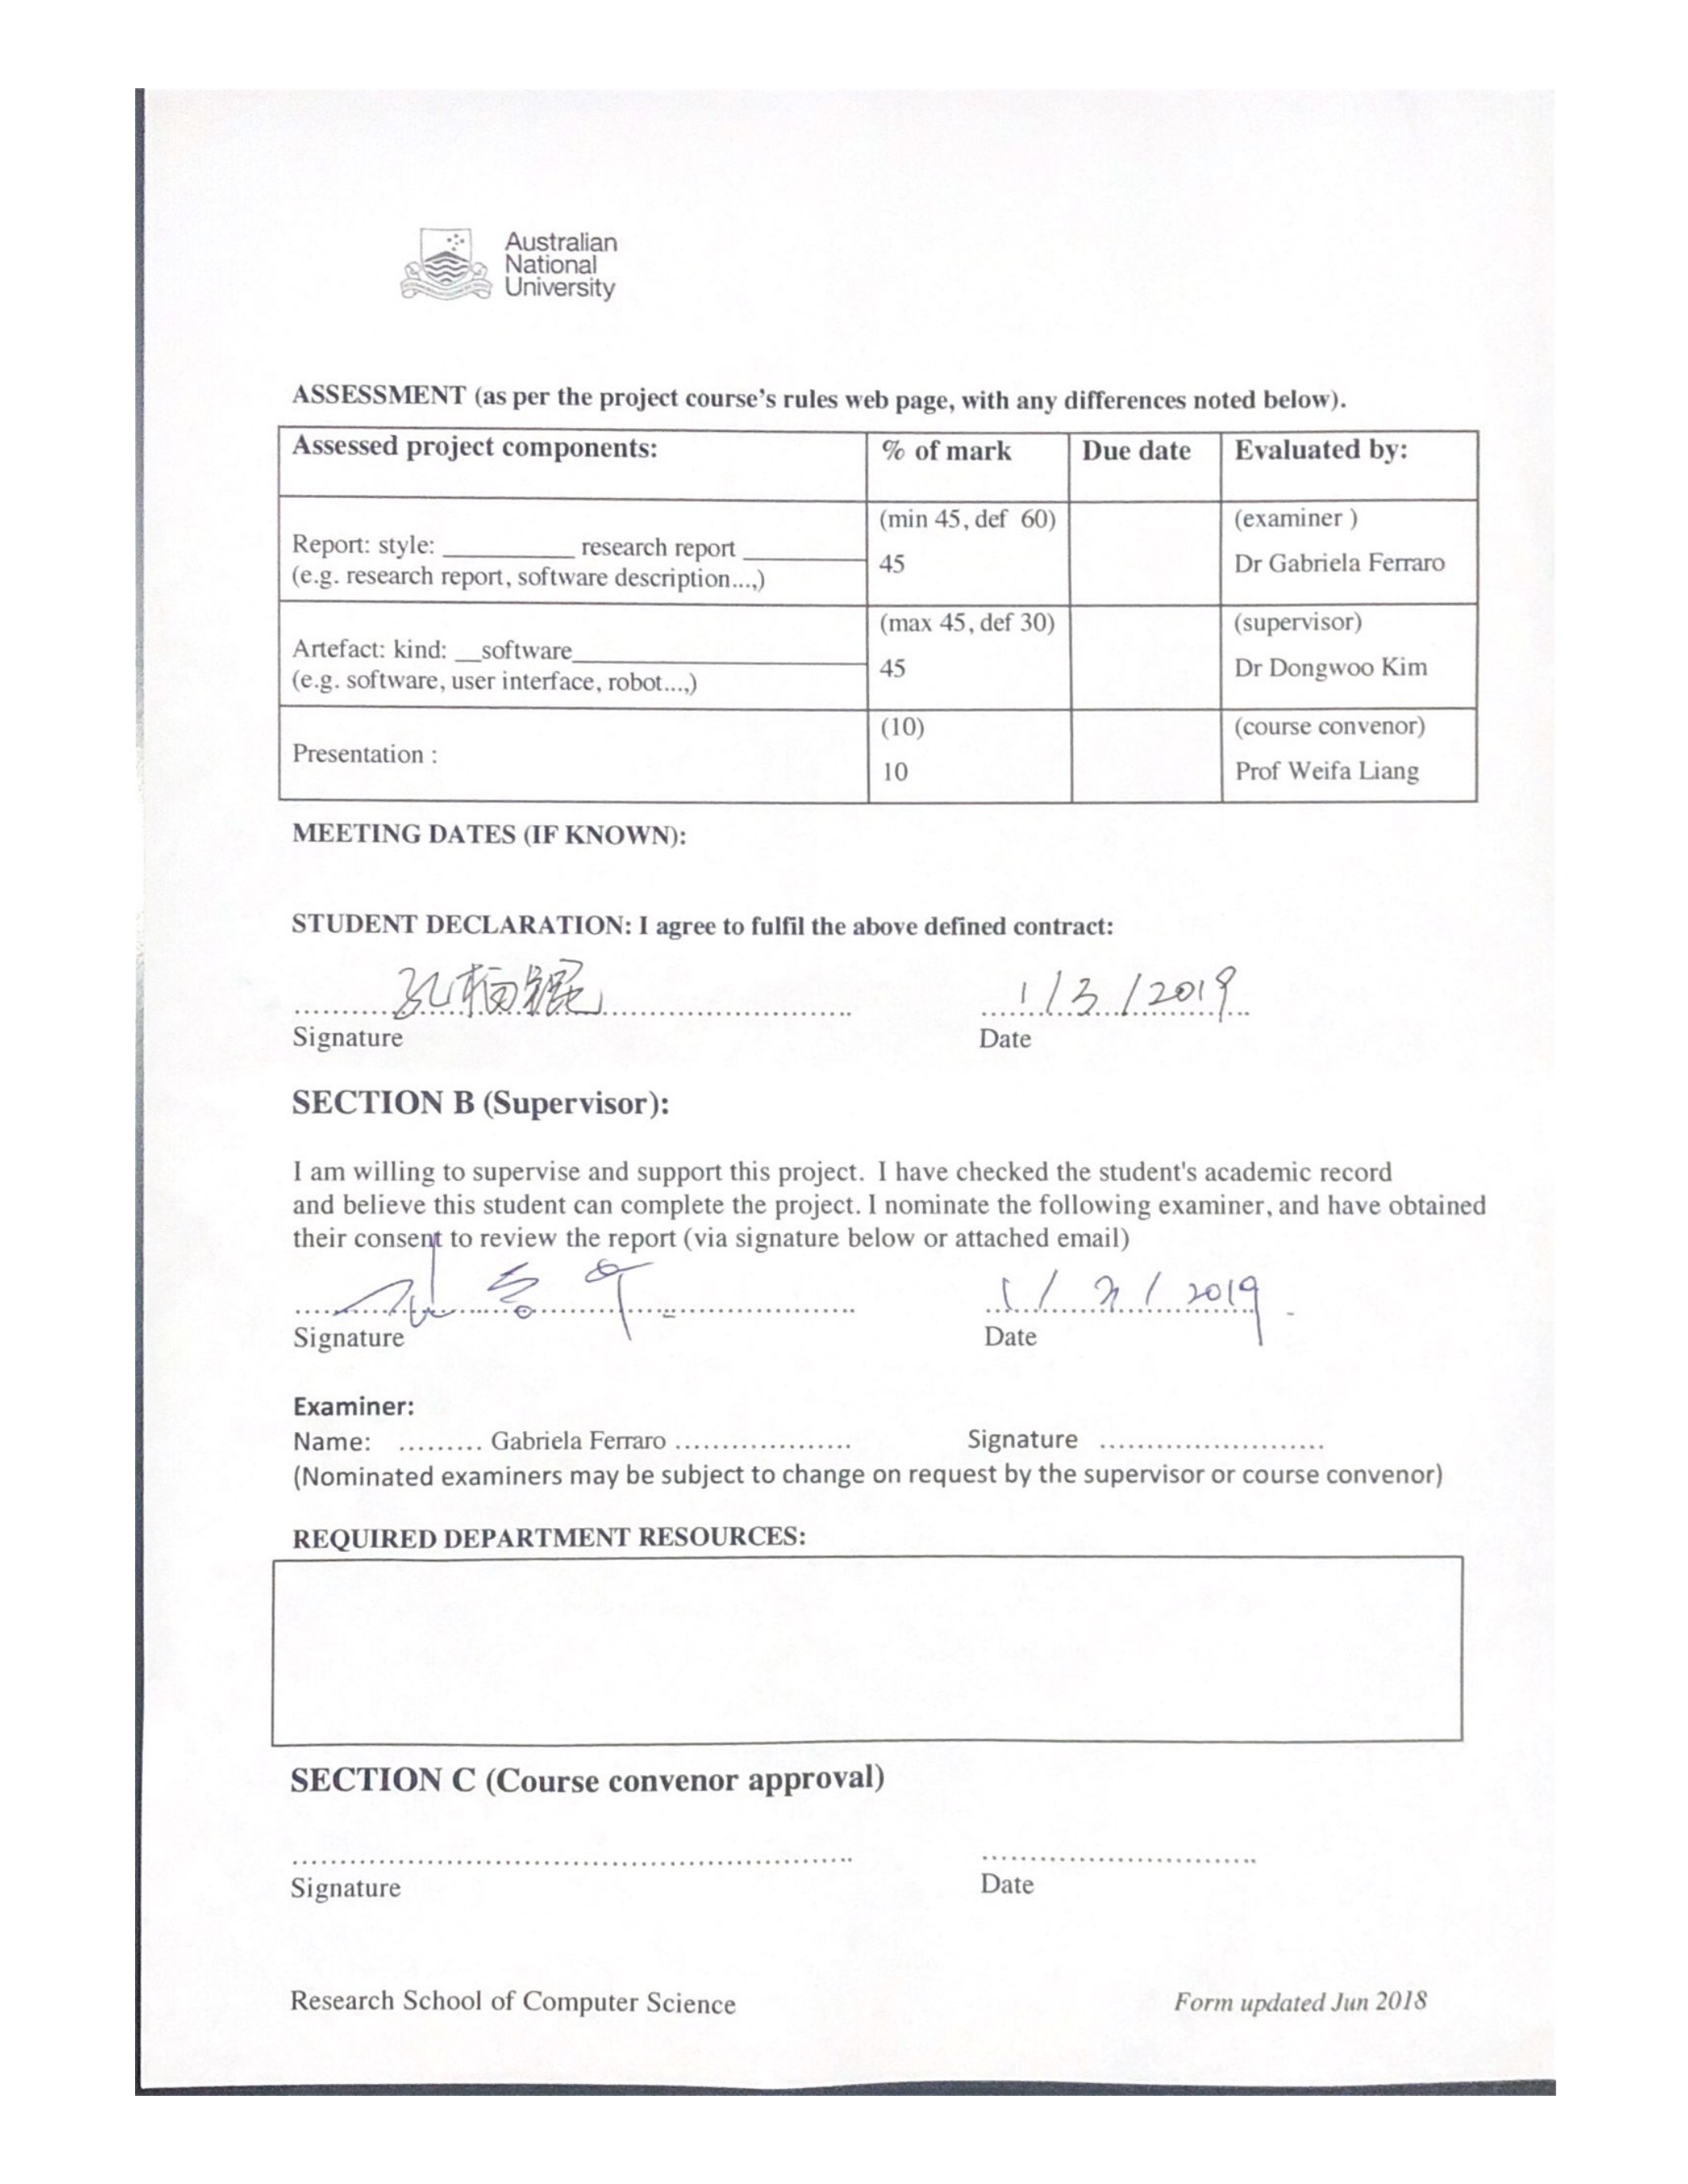}}
	\caption{Independent study contract.}
	\label{fig:ct2}
\end{figure}
